# Supplementary material for: Interlayer exciton dynamics in van der Waals heterostructures
Source: arXiv:1804.08412 ancillary file (2018-04-23)
Supplement: Supplementary file 1 [file Supplementary_20-04-2018.pdf]

# Supplementary material
# Interlayer exciton dynamics in van der Waals heterostructures

Simon Ovesen[1],* Samuel Brem[1], Christopher Linderälv[1], Mikael Kuisma[1,2], Paul Erhart[1], Malte Selig[3], and Ermin Malic[1]
[1] *Chalmers University of Technology, Department of Physics, 41296 Gothenburg, Sweden*
[2] *University of Jyväskylä, Department of Chemistry, Nanoscience Center, 40014 Jyväskylä, Finland and*
[3] *Technical University Berlin, Institute of Theoretical Physics, 10623 Berlin, Germany*

## I. EFFECTIVE 2D COULOMB POTENTIAL

To derive an effective 2D Coulomb potential we model the heterostructure as two aligned homogeneous slabs with the thicknesses $d_{1,2}$, infinite reach in the in-plane direction, and the dielectric constants $\varepsilon_{l_{1,2}}$. They are surrounded by dielectric media characterized by $\varepsilon_{1,2}$ and separated by a distance $R$, in which the medium has the permittivity $\varepsilon_R$. In the middle of layer 2 a point charge $e_0$ is placed. By performing the Fourier transforming in the in-plane direction, the Poisson equation can then be expressed as

$$\left(-k^2 + \frac{\partial^2}{\partial z^2}\right) V(k,z) = -\frac{e_0^2}{\varepsilon_0 \varepsilon_{l_2}} \delta(z). \tag{1}$$

Here, $k$ is the in-plane momentum and $V(k,z)$ is the Coulomb potential. We search for a Coulomb potential that can be expressed as $V_k^{ll'}$, where the indices $l, l'$ describe the layer of the two charges involved. By solving Eq. (1) within the two slabs and neglecting the in-layer $z$ dependence, the solution gives us access to $V_k^{l_2 l_1}$ and $V_k^{l_2 l_2}$. By performing these steps we find that

$$V_k^{ll'} = \frac{e_0^2}{k \varepsilon_0 \varepsilon^{ll'}(k)}, \tag{2}$$

where $\varepsilon^{ll'}(k)$ is the dielectric function of the system. For the interlayer case it has the form

$$\varepsilon^{l_2 l_1}(k) = \cosh(kR) \frac{\cosh(kd_1)\cosh(kd_2)}{\cosh\left(k\frac{d_1}{2}\right)\cosh\left(k\frac{d_2}{2}\right)\left(1+\frac{\varepsilon_1}{\varepsilon_{l_1}}\tanh\left(k\frac{d_1}{2}\right)\right)\left(1+\frac{\varepsilon_2}{\varepsilon_{l_2}}\tanh\left(k\frac{d_2}{2}\right)\right)} f(k), \tag{3}$$

with

$$\begin{aligned} f(k) = &\left((\varepsilon_1+\varepsilon_2) + \left(\frac{\varepsilon_1\varepsilon_2}{\varepsilon_R} + \varepsilon_R\right)\tanh(kR)\right) \\ &+ \left(\left(\varepsilon_{l_1} + \frac{\varepsilon_1\varepsilon_2}{\varepsilon_{l_1}}\right) + \left(\frac{\varepsilon_{l_1}\varepsilon_2}{\varepsilon_R} + \frac{\varepsilon_1\varepsilon_R}{\varepsilon_{l_1}}\right)\tanh(kR)\right)\tanh(kd_1) \\ &+ \left(\left(\varepsilon_{l_2} + \frac{\varepsilon_1\varepsilon_2}{\varepsilon_{l_2}}\right) + \left(\frac{\varepsilon_{l_2}\varepsilon_1}{\varepsilon_R} + \frac{\varepsilon_2\varepsilon_R}{\varepsilon_{l_2}}\right)\tanh(kR)\right)\tanh(kd_2) \\ &+ \left(\left(\frac{\varepsilon_{l_2}}{\varepsilon_{l_1}}\varepsilon_1 + \frac{\varepsilon_{l_1}}{\varepsilon_{l_2}}\varepsilon_2\right) + \left(\frac{\varepsilon_{l_1}\varepsilon_{l_2}}{\varepsilon_R} + \frac{\varepsilon_1\varepsilon_2}{\varepsilon_{l_1}\varepsilon_{l_2}}\varepsilon_R\right)\tanh(kR)\right)\tanh(kd_1)\tanh(kd_2). \end{aligned} \tag{4}$$

This expression diverges for $R \to \infty$ and the potential vanishes. The same result is obtained for $\varepsilon_R \to \infty$. In the limit $R \to 0$ it reduces to $(\varepsilon_1 + \varepsilon_2) + k(\varepsilon_{l_1} d_1 + \varepsilon_{l_2} d_2)$ after linearizing and assuming $\varepsilon_{1,2,R} \ll \varepsilon_{l_{1,2}}$. This is the Keldysh dielectric function for a single layer of the thickness $d_1 + d_2$ and a dielectric constant $\frac{\varepsilon_{l_1} d_1 + \varepsilon_{l_2} d_2}{d_1 + d_2}$. Finally the expression also diverges for $k \to \infty$. To motivate this we consider the simpler case of two particles in a vacuum, separated by $\sqrt{r^2 + z^2}$, where $\mathbf{r}$ and $z$ are in- and out-of-plane coordinates in an arbitrary coordinate system. After

* simon.ovesen@chalmers.se

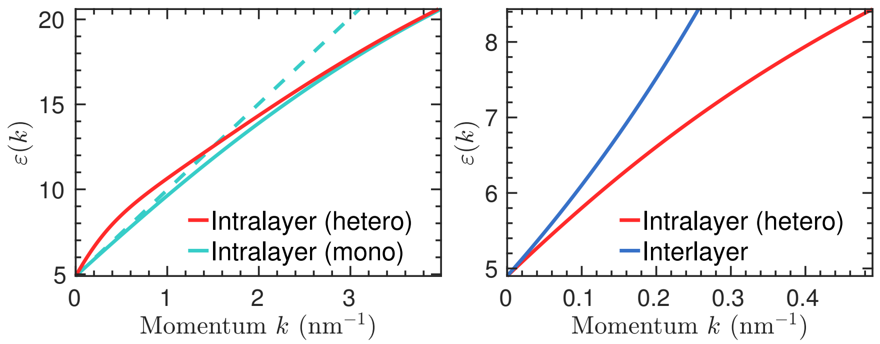


**Figure 1**. **VdW heterostructure dielectric functions.** The dielectric function $\varepsilon(q)$ for the (a) intralayer case in a monolayer and within a heterostructure and the (b) intra- and interlayer case within a heterostructure. The Keldysh limit describes the dielectric function after linearization and assuming that the dielectric constants are significantly larger than those of the surrounding media.

Fourier transforming **r** the corresponding Coulomb potential becomes $V(k,z) \propto \frac{1}{k}\int_0^\infty ds \frac{s}{\sqrt{s^2+k^2z^2}} J_0(s)$, where $J_0(s)$ is the zeroth order Bessel function of the first kind. This can be interpreted as the 2D Coulomb potential with an effective screening $1/\left(\int_0^\infty ds \frac{s}{\sqrt{s^2+k^2z^2}} J_0(s)\right)$, a screening that diverges for $k \to \infty$.

For the intralayer case the result reads

$$\varepsilon^{l_2 l_2}(k) = \frac{\cosh(kd_2)}{\cosh^2\left(k\frac{d_2}{2}\right)\left(1+\tanh\left(k\frac{d_2}{2}\right)\frac{\varepsilon_2}{\varepsilon_{l_2}}\right)} f(k)/ \\ /\left[\left(1+\frac{\varepsilon_1}{\varepsilon_R}\tanh(kR)\right)+\left(\frac{\varepsilon_1}{\varepsilon_{l_1}}+\frac{\varepsilon_{l_1}}{\varepsilon_R}\tanh(kR)\right)\tanh(kd_1)\right. \\ \left.+\left(\frac{\varepsilon_1}{\varepsilon_{l_2}}+\frac{\varepsilon_R}{\varepsilon_{l_2}}\tanh(kR)\right)\tanh\left(k\frac{d_2}{2}\right)+\left(\frac{\varepsilon_{l_1}}{\varepsilon_{l_2}}+\frac{\varepsilon_1\varepsilon_R}{\varepsilon_{l_1}\varepsilon_{l_2}}\tanh(kR)\right)\tanh(kd_1)\tanh\left(k\frac{d_2}{2}\right)\right].$$

For $k \to 0$, we obtain $\varepsilon_1 + \varepsilon_2$, which is consistent with the Keldysh case, while $k \to \infty$ results in $\varepsilon_{l_2}$. When $\varepsilon_1 = \varepsilon_{l_1} = \varepsilon_R$ the $R$ dependence completely vanishes, and for $\varepsilon_{1,2} \ll \varepsilon_{l_2}$ results in the ordinary Keldysh dielectric function after linearization. The limit $R \to \infty$ results in the same, but with $\varepsilon_R$ taking the role of $\varepsilon_1$.

Figure 1(a) shows a comparison of the dielectric function $\varepsilon(q)$ for the intralayer case in a monolayer and within a heterostructure, while Fig. 1(b) displays the comparison between intra- and interlayer cases within a heterostructure. As parameters we have used $d_{1,2} = a_0^{1,2}$ and $R = \frac{d_1+d_2}{2}$, where $a_0^l$ is the lattice constant for the layer $l$, i.e. $l_{1,2}$ representing $WSe_2$ and $MoSe_2$ layers. For the dielectric constants, we have assumed $\varepsilon_{1,R} = 1$ and $\varepsilon_2 = 3.9$ representing air and $SiO_2$, as well as $\varepsilon_{l_1} = 13.63$ and $\varepsilon_{l_2} = 15.27$ for $WSe_2$ and $MoSe_2$.

## II. EXCITONIC WAVEFUNCTIONS AND LUMINESCENCE BLOCH EQUATIONS

The excitonic wavefunctions are obtained through solving the Wannier equations, cf. Fig. 2. A general trend that can be observed is that a lower binding energy leads to sharper excitonic wavefunctions in the momentum space corresponding to more delocalized excitonic states in the real space. A consequence of this is that interactions involving interlayer excitons will favor scattering events with lower momentum transfers.

The luminescence Bloch equations shown in the main text can be more explicitly expressed as

$$\dot{P}_{\boldsymbol{Q}}^{l_h l_e} = \frac{1}{i\hbar} E_{\boldsymbol{Q}}^{l_h l_e} P_{\boldsymbol{Q}}^{l_h l_e} + i\Omega_{\boldsymbol{Q}}^{l_h l_e} - \left(\gamma_r^{l_h l_e} + \frac{1}{2}\sum_{\boldsymbol{Q}'} \Gamma_{P,\boldsymbol{Q}\boldsymbol{Q}'}^{l_h l_e}\right) P_{\boldsymbol{Q}}^{l_h l_e} \tag{5}$$

$$\dot{N}_{\boldsymbol{Q}}^{l_h l_e} = \sum_{\boldsymbol{Q}'} \Gamma_{P,\boldsymbol{Q}'\boldsymbol{Q}}^{l_h l_e} |P_{\boldsymbol{Q}'}^{l_h l_e}|^2 - 2\gamma_r^{l_h l_e}\delta_{\boldsymbol{Q},0} N_{\boldsymbol{Q}}^{l_h l_e} + \sum_{\boldsymbol{Q}'} (\Gamma_{P,\boldsymbol{Q}'\boldsymbol{Q}}^{l_h l_e} N_{\boldsymbol{Q}'}^{l_h l_e} - \Gamma_{P,\boldsymbol{Q}\boldsymbol{Q}'}^{l_h l_e} N_{\boldsymbol{Q}}^{l_h l_e}) \\ + \sum_{\boldsymbol{Q}' l_h' l_e'} \Gamma_{T,\boldsymbol{Q}\boldsymbol{Q}'}^{l_h l_e l_h' l_e'} (N_{\boldsymbol{Q}'}^{l_h' l_e'} - N_{\boldsymbol{Q}}^{l_h l_e}). \tag{6}$$

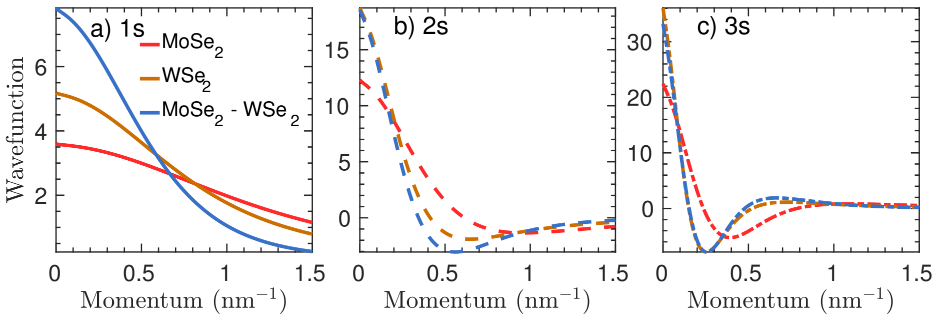


**Figure 2**. **Exciton wavefunctions.** Wavefunctions of the lowest exciton states (1s, 2s, and 3s) for the $MoSe_2$ and $WSe_2$ intralayer excitons and the corresponding $MoSe_2$-$WSe_2$ interlayer exciton, respectively.

The first two terms describing the dynamics of the exciton polarization $P_{\boldsymbol{Q}}^{l_h l_e}(t)$ with hole (electron) in the layer $l_h$ ($l_e$) are determined by the excitonic dispersion $E_{\boldsymbol{Q}}^{l_h l_e}$ and the Rabi frequency $\Omega_{\boldsymbol{Q}}^{l_h l_e}(t) = i\frac{e_0}{m_0}\sum_{\boldsymbol{q}} \varphi_{\boldsymbol{q}}^{*l_h l_e} \boldsymbol{M}_{\boldsymbol{q}}^{l_h l_e} \cdot \boldsymbol{A}(t)$. Here, $e_0$ and $m_0$ are the elementary charge and electronic rest mass, $\varphi_{\boldsymbol{q}}^{l_h l_e}$ is the excitonic wavefunction, $\boldsymbol{M}_{\boldsymbol{q}}^{l_h l_e}$ the optical matrix element describing optical interband transitions [1, 2] and $\boldsymbol{A}(t)$ is the driving optical pump pulse. The decay processes stem from the radiative damping is described by the rate $\gamma_r^{l_h l_e} = \frac{\hbar^2 c_0 \mu_0}{\omega^{l_h l_e} n} \left| \sum_{\boldsymbol{q}} \varphi_{\boldsymbol{q}}^{*l_h l_e} M_{\boldsymbol{q}}^{l_h l_e} \right|^2$, where $\frac{c_0}{n}$ is the speed of light in the substrate material, $\mu_0$ the vacuum permeability and $\omega^{l_h l_e}$ the resonant photon frequency [2]. The exciton-phonon interaction is determined by the rate $\Gamma_{P,\boldsymbol{Q},\boldsymbol{Q}'}^{l_h l_e} = \frac{2\pi}{\hbar}\sum_{l\alpha\pm} |G_{\boldsymbol{Q}-\boldsymbol{Q}'}^{l_h l_e l\alpha}|^2 \hat{n}_{\boldsymbol{Q}-\boldsymbol{Q}'}^{l\alpha\pm} \delta(\Delta E_{\boldsymbol{Q},\boldsymbol{Q}'}^{l_h l_e l\alpha\pm})$, where the scattering cross section is given by $G_{\boldsymbol{K}}^{l_h l_e l\alpha} = \sum_{\boldsymbol{q}} \varphi_{\boldsymbol{q}}^{*l_h l_e} \left( \varphi_{\boldsymbol{q}+\beta^{l_h l_e}\boldsymbol{K}}^{l_h l_e} g_{\boldsymbol{K}}^{c,l_e\alpha} \delta^{l_e l} - \varphi_{\boldsymbol{q}-\alpha^{l_h l_e}\boldsymbol{K}}^{l_h l_e} g_{\boldsymbol{K}}^{v,l_h\alpha} \delta^{l_h l} \right)$. Here, $\alpha^{l_h l_e} = \frac{m_e^{l_e}}{m_h^{l_h} + m_e^{l_e}}$ and $\beta^{l_h l_e} = \frac{m_h^{l_h}}{m_h^{l_h} + m_e^{l_e}}$ and $g^{\lambda,l\alpha}$ is the electron-phonon matrix element for band $\lambda$ (with $c$ and $v$ denoting the conduction and valence bands), layer $l$ and phonon mode $\alpha$. Furthermore, $\Delta E_{\boldsymbol{Q},\boldsymbol{Q}'}^{l_h l_e l\alpha\pm} = E_{\boldsymbol{Q}'}^{l_h l_e} - E_{\boldsymbol{Q}}^{l_h l_h} \pm \hbar\omega_{\boldsymbol{Q}-\boldsymbol{Q}'}^{l\alpha}$ describes the energy difference when absorbing ($-$) or emitting ($+$) a phonon with the energy $\hbar\omega_{\boldsymbol{Q}-\boldsymbol{Q}'}^{l\alpha}$. Finally, $\hat{n}_{\boldsymbol{Q}-\boldsymbol{Q}'}^{l\alpha\pm} = \frac{1}{2} \pm \frac{1}{2} + n_{\boldsymbol{Q}-\boldsymbol{Q}'}^{l\alpha}$, where the phonon occupation $n_K^{l\alpha} = \frac{1}{\exp\left(\frac{\hbar\omega_{\boldsymbol{K}}^{l\alpha}}{k_B T}\right) - 1}$ with Boltzmann constant $k_B$ and temperature $T$ is treated as a Bose-Einstein distribution [2, 3].

The dynamics of the incoherent exciton occupation $N_{\boldsymbol{Q}}^{l_h l_e}(t)$ is determined by formation processes driven by phonon-assisted decay of the excitonic polarization, the radiative decay, and exciton-phonon scattering driving the excited system towards an equilibrium Boltzmann-like distribution [3, 4]. The final term in Eq. (6) describes resonant tunneling between different layers and causes the formation of interlayer excitons. It has an effective scattering rate $\Gamma_{T,\boldsymbol{Q}\boldsymbol{Q}'}^{l_h l_e l'_h l'_e} = \frac{2\pi}{\hbar} |\tilde{T}_{\boldsymbol{Q}\boldsymbol{Q}'}^{l_h l_e l'_h l'_e}|^2 \delta(E_{\boldsymbol{Q}'}^{l'_h l'_e} - E_{\boldsymbol{Q}}^{l_h l_e})$, where the exciton tunneling cross section is expressed as $\tilde{T}_{\boldsymbol{Q}\boldsymbol{Q}'}^{l_h l_e l'_h l'_e} = \sum_{\boldsymbol{q}} \left( \varphi_{\boldsymbol{q}+\beta^{l_h l_e}\boldsymbol{Q}}^{*l_h l_e} \varphi_{\boldsymbol{q}+\beta^{l'_h l'_e}\boldsymbol{Q}'}^{l'_h l'_e} T_{\boldsymbol{q}+\boldsymbol{Q},\boldsymbol{q}+\boldsymbol{Q}'}^{c,l_e l'_e} (1 - \delta^{l_e l'_e}) \delta^{l_h l'_h} - \varphi_{\boldsymbol{q}-\alpha^{l_h l_e}\boldsymbol{Q}}^{*l_h l_e} \varphi_{\boldsymbol{q}-\alpha^{l'_h l'_e}\boldsymbol{Q}'}^{l'_h l'_e} T_{\boldsymbol{q}-\boldsymbol{Q},\boldsymbol{q}-\boldsymbol{Q}'}^{*v,l_h l'_h} \delta^{l_e l'_e} (1 - \delta^{l_h l'_h}) \right)$. Here $T_{\boldsymbol{K},\boldsymbol{K}'}^{\lambda,ll'} = \frac{\sqrt{\pi} L_c}{\left(1 + \frac{|\boldsymbol{K}' - \boldsymbol{K}|^2 L_C^2}{2}\right)^{\frac{3}{4}}} V_z \left\langle u_{\boldsymbol{K}}^{\lambda l} | u_{\boldsymbol{K}}^{\lambda l'} \right\rangle_{\text{uc}}$ is the electron tunneling matrix element that has been discussed in the main text.

## III. DFT CALCULATIONS

The structure consisting of a $MoSe_2$ and a $WSe_2$ layer in a 2H configuration was relaxed in the software VASP [5] with both PBE and vdW-DF-cx until the maximal force was 5 meV/Å. The plane wave cutoff energy was 300 eV and the Brillouin zone was sampled with a $15 \times 15 \times 5$ **k**-point mesh. The PBE bilayer (with in-plane lattice constant 3.32 Å) was then isolated and a vacuum of 10 Å was applied to the bilayer. One monolayer was then shifted such that the Mo-W distance matched the value obtained from the relaxation with the vdW-DF-cx functional (6.45 Å). The bilayer system was then split up into two configurations consisting of a single layer. The wavefunctions of the separate layers were then computed on a real space grid with GPAW [6] using norm conserving potentials and a grid spacing of 0.2 $Å^{-1}$. The **k**-point mesh for the self-consistent calculation of the electron density was $33 \times 33 \times 1$. The wavefunctions were then computed on a radial grid centered at K that extended 0.4 $Å^{-1}$. The radial grid consisted of 25 radial points (including K) and 40 angular points. The value of the overlap integral (for a smaller k-point set) was checked with a reduced grid spacing of 0.1 $Å^{-1}$.

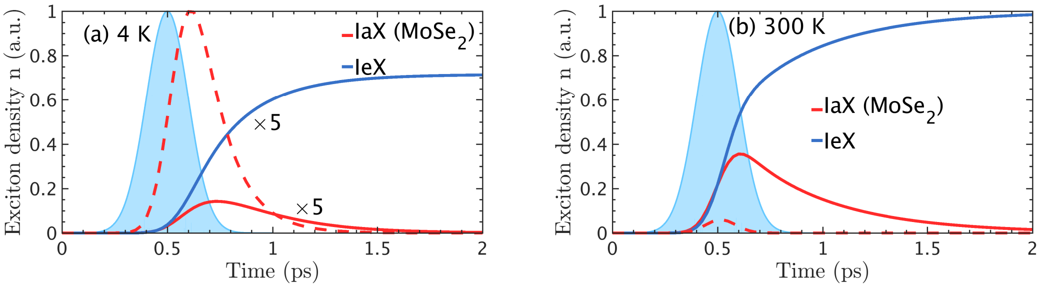


**Figure 3**. **Momentum-integrated exciton dynamics.** Evolution of the $MoSe_2$ intralayer (IaX) and interlayer (IeX) 1s exciton densities $n$ after resonant optical excitation of the $MoSe_2$ layer at (a) 4 K and (b) 300 K (b). The optical pulse is denoted by the blue-shaded Gaussian. The dashed line represents coherent excitons in the $MoSe_2$ layer.

## IV. TEMPERATURE DEPENDENCE OF EXCITON DYNAMICS

While in the main text, intra- and interlayer exciton dynamics and photoluminescence has been shown at 77 K, here we present the momentum integrated dynamics calculated at 4 K and 300 K. Figure 3 shows how the coherence lifetime drastically increases at very low temperatures, which can be seen by comparing the red dashed lines in Fig. 3(a) and Fig. 3(b). This behavior can be traced back to the reduced efficiency of exciton-phonon scattering, which also explains the less pronounced polarization-to-population transfer, i.e. the formation of incoherent excitons (red solid lines). This has a direct impact on the photoluminescence, which is presented in Fig. 4. At 4 K (Fig. 4(a - c)) exciton-phonon scattering becomes significantly less efficient than interlayer tunneling. As a result, there is a non-negligible delay until interlayer excitons scatter into the light cone and become visible in PL. As a result, the IeX emission does not saturate after surpassing the IaX resonance at 4.7 ps (blue line in Fig. 4(b)). Instead it slowly increases until it reaches equilibrium at approximately 50 ps (purple line in Fig. 4(b)). This increase can be seen in more detail in Figs. 4(a, c). At 300 K (Fig. 4(d - f)) the IeX resonance can barely be seen due to the broadening of the intralayer exciton transition. This can be well seen in Fig. 4(f). In contrast to 4 K and 77 K, the total emission at the IeX energy including off-resonant IaX emission (dashed blue line) exceeds the emission from IeX alone (solid blue line).

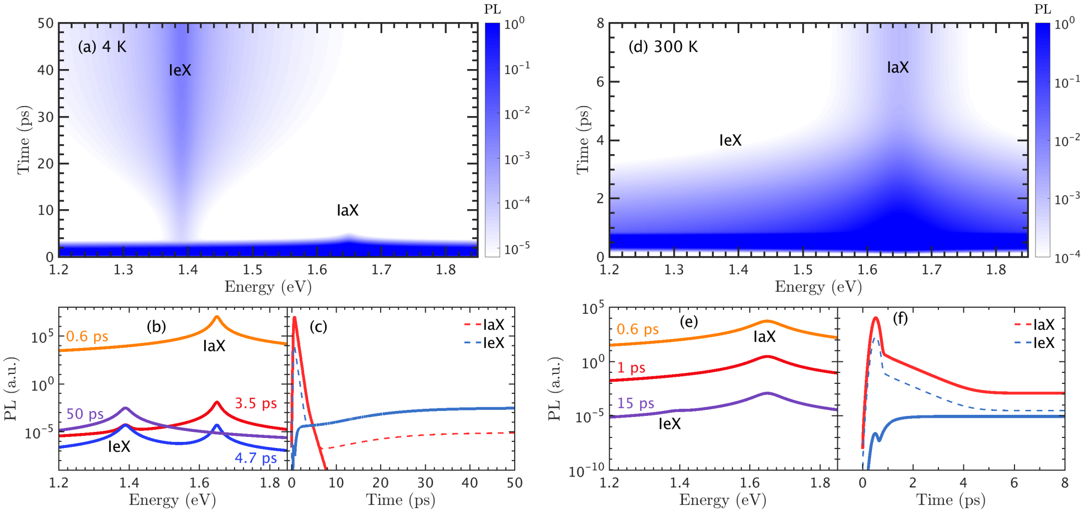


**Figure 4**. **Time- and energy-resolved photoluminescence.** PL of the investigated heterostructure at 4 K (a-c) and 300 K (d-f) plotted (a, d) over time and energy (logarithmic) and showing snapshots taken at specific (b, e) times and (c, f) energies. The chosen energies correspond to the position of the interlayer (IeX) and $MoSe_2$ intralayer (IaX) exciton resonance, respectively. The dashed lines in (c, f) represent the signals stemming from the inter- or intralayer emission only, while the dashed lines also include the spectral overlap with the respective other peak.

[1] G. Berghäuser and E. Malic, Phys. Rev. B **89**, 125309 (2013).
[2] M. Selig, G. Berghäuser, A. Raja, P. Nagler, C. Schüller, T. F. Heinz, T. Korn, A. Chernikov, E. Malic, and A. Knorr, Nat Commun. **7** (2016).
[3] S. Brem, G. Berghaeuser, M. Selig, and E. Malic, (2017), arXiv:1712.04808.
[4] M. Selig, G. Berghäuser, M. Richter, R. Bratschitsch, A. Knorr, and E. Malic, (2017), arXiv:1703.03317.
[5] G. Kresse and J. Furthmüller, Comp. Mater. Sci. **6**, 15 (1996).
[6] J. Enkovaara, C. Rostgaard, J. J. Mortensen, J. Chen, M. Du-ak, L. Ferrighi, J. Gavnholt, C. Glinsvad, V. Haikola, H. A. Hansen, H. H. Kristoffersen, M. Kuisma, A. H. Larsen, L. Lehtovaara, M. Ljungberg, O. Lopez-Acevedo, P. G. Moses, J. Ojanen, T. Olsen, V. Petzold, N. A. Romero, J. Stausholm-Møller, M. Strange, G. A. Tritsaris, M. Vanin, M. Walter, B. Hammer, H. Häkkinen, G. K. H. Madsen, R. M. Nieminen, J. K. Nørskov, M. Puska, T. T. Rantala, J. Schiøtz, K. S. Thygesen, and K. W. Jacobsen, Journal of Physics: Condensed Matter **22**, 253202 (2010).
